# Supplementary material for: Application of the Brain Drain Optimization Algorithm to the N-Queens Problem
Source: arXiv:2504.18953 source file (2025-04-26)
Supplement: Supplementary file 1 [file main.tex]

\documentclass[pdflatex,sn-mathphys-num]{sn-jnl}% Math and Physical Sciences Numbered Reference Style
\usepackage{amssymb}
\usepackage{amsmath}
\usepackage{float}
\usepackage{comment}
\usepackage{multirow}
\usepackage{natbib}
\usepackage{booktabs}   % beautiful rules
\usepackage{siunitx}    % aligned numbers
\usepackage{rotating}   % sidewaystable
\usepackage{tabularx}   % (optional) automatic column width
\usepackage{algorithm}
\usepackage{algpseudocode}
\usepackage{float}

\begin{document}

\title{Supplementary Information for "Application of the Brain Drain Optimization Algorithm to the N-Queens Problem"}
\maketitle

\section{Overview of Parameter Settings}

Table \ref{tab:algorithm_parameters} represents the parameter settings considered for tuning each algorithm evaluated in this study. For each algorithm, a set of key parameters and their respective candidate values are listed, enabling the best configuration during the experiments. The parameter ranges have been selected based on preliminary experiments.

\begin{table}[!htb]
    \centering
    \small
    \setlength{\tabcolsep}{4pt}
    \setlength{\tabcolsep}{4pt} % Shrink horizontal space
    \renewcommand{\arraystretch}{0.9} % Shrink row height
    \begin{tabular}{p{2cm} p{11cm}} % Two columns: Algorithm Name & Parameter Settings
        \toprule
        \textbf{Algorithm} & \textbf{Parameter Settings} \\
        \midrule
        \multirow{8}{*}{BRADO}  
        & Threshold parameter ($\alpha$): \{10, 15, 20, 25\} \\
        & Weight of best neighbors (WG): \{0.6, 0.7, 0.8, 0.9\} \\
        & Distance from worst destination node (D): \{0.1, 0.15, 0.2, 0.25\} \\
        & Initial population ($P_0$): \{30, 50, 70, 90\} \\
        & Probability P in ER model (P): \{0.6, 0.7, 0.8, 0.9\} \\
        & Probability of returning to country (P): \{0.1, 0.2\} \\
        & Initial number of countries (N): \{5, 6, 7, 8\} \\
        & Maximum iterations without improvement: \{30, 70, 100, 150\} \\
        \midrule
        \multirow{4}{*}{GA}  
        & Maximum iterations without improvement: \{30, 70, 100, 150\} \\
        & Initial population: \{30, 50, 80, 100\} \\
        & Crossover probability: \{0.1, 0.2, 0.3, 0.4\} \\
        & Survival rate of the population: \{0.4, 0.5, 0.6, 0.7\} \\
        \midrule
        \multirow{7}{*}{ICA}  
        & Revolution rate values: \{0.2, 0.3, 0.4, 0.5\} \\
        & Uniting threshold values: \{0.01, 0.02, 0.03, 0.04\} \\
        & Zeta values: \{0.01, 0.02, 0.03, 0.04\} \\
        & Population size values: \{70, 80, 90, 100\} \\
        & Assimilation coefficient values: \{1, 2, 3, 4\} \\
        & Number of initial imperialist values: \{5, 6, 7, 8\} \\
        & Maximum iterations without improvement: \{30, 70, 100, 150\} \\
        \midrule
        \multirow{4}{*}{PSO}  
        & Maximum iterations without improvement: \{30, 70, 100, 150\} \\
        & Initial population: \{30, 50, 80, 100\} \\
        & $C$ (cognitive parameter): \{0.5, 1, 1.5, 2\} \\
        & $C$ (social parameter): \{0.5, 1, 1.5, 2\} \\
        \midrule
        \multirow{4}{*}{ILS}  
        & Initial node selection method: \{1, 2\} \\
        & Maximum iterations without improvement: \{30, 70, 100, 150\} \\
        & Perturbation radius for new point: \{0.2, 0.5, 0.8, 1\} \\
        & Number of iterations: \{5, 10, 15, 20\} \\
        \midrule
        \multirow{2}{*}{LS}  
        & Maximum iterations without improvement: \{30, 70, 100, 150\} \\
        & Perturbation radius for new point: \{0.2, 0.5, 0.8, 1\} \\
        \midrule
        \multirow{3}{*}{MLS}  
        & Maximum iterations without improvement: \{30, 70, 100, 150\} \\
        & Perturbation radius for new point: \{0.2, 0.5, 0.8, 1\} \\
        & Number of iterations: \{5, 10, 15, 20\} \\
        \bottomrule
    \end{tabular}
    \caption{Parameter settings for different algorithms}
    \label{tab:algorithm_parameters}
\end{table}


\section{Parameter tuning phase}

After executing the algorithms five times with different parameter levels for each problem ranging from 8 to 1000 variables, the best results were obtained. The optimal parameter level combinations for each problem have been determined and are detailed below.

\begin{table}[!htb]
    \small
    \setlength{\tabcolsep}{4pt}
    \setlength{\tabcolsep}{4pt} % Shrink horizontal space
    \renewcommand{\arraystretch}{0.9} % Shrink row height
    \caption{Best Selected Parameter Levels for Problem with 8 Variables}
    \label{tab:best_parameters_8vars}
    \begin{tabular}{p{2cm} p{11cm}} % Two columns: Algorithm Name & Parameter Settings
        \toprule
        \textbf{Algorithm} & \textbf{Selected Parameter Values Based on the TOPSIS Method} \\
        \midrule
        \multirow{8}{*}{BRADO}  
        & Threshold parameter ($\alpha$): 15 \\
        & Best neighbor weight (WG): 0.8 \\
        & Distance from the worst destination node (D): 0.15 \\
        & Initial population ($P_0$): 90 \\
        & Probability P in ER model: 0.6 \\
        & Probability of returning to origin country: 0.2 \\
        & Number of initial countries: 6 \\
        & Maximum iterations without improvement: 100 \\
        \midrule
        \multirow{4}{*}{GA}  
        & Maximum iterations without improvement: 150 \\
        & Initial population: 50 \\
        & Crossover probability: 0.1 \\
        & Survival rate of the population: 0.6 \\
        \midrule
        \multirow{6}{*}{ICA}  
        & Revolution rate values: 0.4 \\
        & Uniting threshold values: 0.02 \\
        & Zeta values: 0.04 \\
        & Population size values: 90 \\
        & Assimilation coefficient values: 1 \\
        & Number of initial imperialist values: 8 \\
        & Maximum iterations without improvement: 100 \\
        \midrule
        \multirow{4}{*}{ILS}  
        & Initial node selection method: 1 \\
        & Maximum iterations without improvement: 100 \\
        & Perturbation radius for new point: 1 \\
        & Number of iterations: 15 \\
        \midrule
        \multirow{2}{*}{LS}  
        & Maximum iterations without improvement: 150 \\
        & Perturbation radius for new point: 0.8 \\
        \midrule
        \multirow{3}{*}{MLS}  
        & Maximum iterations without improvement: 150 \\
        & Perturbation radius for new point: 1 \\
        & Number of iterations: 20 \\
        \midrule
        \multirow{4}{*}{PSO}  
        & Maximum iterations without improvement: 30 \\
        & Initial population: 100 \\
        & $C$ (cognitive parameter): 1.5 \\
        & $C$ (social parameter): 0.5 \\
        \bottomrule
    \end{tabular}
\end{table}

\begin{table}[!htb]
    \centering
    \small
    \setlength{\tabcolsep}{4pt}
    \setlength{\tabcolsep}{4pt} % Shrink horizontal space
    \renewcommand{\arraystretch}{0.9} % Shrink row height
    \caption{Best Selected Parameter Levels for Problem with 10 Variables}
    \label{tab:best_parameters_10vars}
    \begin{tabular}{p{2cm} p{11cm}} % Two columns: Algorithm Name & Parameter Settings
        \toprule
        \textbf{Algorithm} & \textbf{Selected Parameter Values Based on the TOPSIS Method} \\
        \midrule
        \multirow{8}{*}{BRADO}  
        & Threshold parameter ($\alpha$): 20 \\
        & Best neighbor weight (WG): 0.7 \\
        & Distance from the worst destination node (D): 0.1 \\
        & Initial population ($P_0$): 90 \\
        & Probability P in ER model: 0.6 \\
        & Probability of returning to origin country: 0.2 \\
        & Number of initial countries: 6 \\
        & Maximum iterations without improvement: 150 \\
        \midrule
        \multirow{4}{*}{GA}  
        & Maximum iterations without improvement: 150 \\
        & Initial population: 100 \\
        & Crossover probability: 0.1 \\
        & Survival rate of the population: 0.4 \\
        \midrule
        \multirow{6}{*}{ICA}  
        & Revolution rate values: 0.3 \\
        & Uniting threshold values: 0.01 \\
        & Zeta values: 0.01 \\
        & Population size values: 80 \\
        & Assimilation coefficient values: 1 \\
        & Number of initial imperialist values: 7 \\
        & Maximum iterations without improvement: 150 \\
        \midrule
        \multirow{4}{*}{ILS}  
        & Initial node selection method: 1 \\
        & Maximum iterations without improvement: 70 \\
        & Perturbation radius for new point: 1 \\
        & Number of iterations: 15 \\
        \midrule
        \multirow{2}{*}{LS}  
        & Maximum iterations without improvement: 150 \\
        & Perturbation radius for new point: 1 \\
        \midrule
        \multirow{3}{*}{MLS}  
        & Maximum iterations without improvement: 100 \\
        & Perturbation radius for new point: 1 \\
        & Number of iterations: 20 \\
        \midrule
        \multirow{4}{*}{PSO}  
        & Maximum iterations without improvement: 100 \\
        & Initial population: 100 \\
        & $C$ (cognitive parameter): 1 \\
        & $C$ (social parameter): 0.5 \\
        \bottomrule
    \end{tabular}
\end{table}

\begin{table}[!htb]
    \centering
    \small
    \setlength{\tabcolsep}{4pt}
    \setlength{\tabcolsep}{4pt} % Shrink horizontal space
    \renewcommand{\arraystretch}{0.9} % Shrink row height
    \caption{Best Selected Parameter Levels for Problem with 25 Variables}
    \label{tab:best_parameters_25vars}
    \begin{tabular}{p{2cm} p{11cm}} % Two columns: Algorithm Name & Parameter Settings
        \toprule
        \textbf{Algorithm} & \textbf{Selected Parameter Values Based on the TOPSIS Method} \\
        \midrule
        \multirow{8}{*}{BRADO}  
        & Threshold parameter ($\alpha$): 20 \\
        & Best neighbor weight (WG): 0.8 \\
        & Distance from the worst destination node (D): 0.1 \\
        & Initial population ($P_0$): 80 \\
        & Probability P in ER model: 0.6 \\
        & Probability of returning to origin country: 0.2 \\
        & Number of initial countries: 7 \\
        & Maximum iterations without improvement: 150 \\
        \midrule
        \multirow{4}{*}{GA}  
        & Maximum iterations without improvement: 150 \\
        & Initial population: 30 \\
        & Crossover probability: 0.1 \\
        & Survival rate of the population: 0.4 \\
        \midrule
        \multirow{6}{*}{ICA}  
        & Revolution rate values: 0.3 \\
        & Uniting threshold values: 0.1 \\
        & Zeta values: 0.03 \\
        & Population size values: 70 \\
        & Assimilation coefficient values: 1 \\
        & Number of initial imperialist values: 6 \\
        & Maximum iterations without improvement: 100 \\
        \midrule
        \multirow{4}{*}{ILS}  
        & Initial node selection method: 1 \\
        & Maximum iterations without improvement: 100 \\
        & Perturbation radius for new point: 0.8 \\
        & Number of iterations: 20 \\
        \midrule
        \multirow{2}{*}{LS}  
        & Maximum iterations without improvement: 150 \\
        & Perturbation radius for new point: 0.8 \\
        \midrule
        \multirow{3}{*}{MLS}  
        & Maximum iterations without improvement: 150 \\
        & Perturbation radius for new point: 1 \\
        & Number of iterations: 15 \\
        \midrule
        \multirow{4}{*}{PSO}  
        & Maximum iterations without improvement: 70 \\
        & Initial population: 100 \\
        & $C$ (cognitive parameter): 1.5 \\
        & $C$ (social parameter): 0.5 \\
        \bottomrule
    \end{tabular}
\end{table}
\begin{table}[!htb]
    \centering
    \small
    \setlength{\tabcolsep}{4pt}
    \setlength{\tabcolsep}{4pt} % Shrink horizontal space
    \renewcommand{\arraystretch}{0.9} % Shrink row height
    \caption{Best Selected Parameter Levels for Problem with 50 Variables}
    \label{tab:best_parameters_50vars}
    \begin{tabular}{p{2cm} p{11cm}} % Two columns: Algorithm Name & Parameter Settings
        \toprule
        \textbf{Algorithm} & \textbf{Selected Parameter Values Based on the TOPSIS Method} \\
        \midrule
        \multirow{8}{*}{BRADO}  
        & Threshold parameter ($\alpha$): 20 \\
        & Best neighbor weight (WG): 0.8 \\
        & Distance from the worst destination node (D): 0.1 \\
        & Initial population ($P_0$): 70 \\
        & Probability P in ER model: 0.8 \\
        & Probability of returning to origin country: 0.1 \\
        & Number of initial countries: 5 \\
        & Maximum iterations without improvement: 150 \\
        \midrule
        \multirow{4}{*}{GA}  
        & Maximum iterations without improvement: 150 \\
        & Initial population: 30 \\
        & Crossover probability: 0.1 \\
        & Survival rate of the population: 0.4 \\
        \midrule
        \multirow{7}{*}{ICA}  
        & Revolution rate values: 0.2 \\
        & Uniting threshold values: 0.01 \\
        & Zeta values: 0.03 \\
        & Population size values: 80\\
        & Assimilation coefficient values: 1 \\
        & Number of initial imperialist values: 6 \\
        & Maximum iterations without improvement: 150 \\
        \midrule
        \multirow{4}{*}{ILS}  
        & Initial node selection method: 1 \\
        & Maximum iterations without improvement: 150 \\
        & Perturbation radius for new point: 0.8 \\
        & Number of iterations: 15 \\
        \midrule
        \multirow{2}{*}{LS}  
        & Maximum iterations without improvement: 70 \\
        & Perturbation radius for new point: 0.8 \\
        \midrule
        \multirow{3}{*}{MLS}  
        & Maximum iterations without improvement: 150 \\
        & Perturbation radius for new point: 1 \\
        & Number of iterations: 20 \\
        \midrule
        \multirow{4}{*}{PSO}  
        & Maximum iterations without improvement: 70 \\
        & Initial population: 100 \\
        & $C$ (cognitive parameter): 2 \\
        & $C$ (social parameter): 0.5 \\
        \bottomrule
    \end{tabular}
\end{table}

\begin{table}[!htb]
    \centering
    \small
    \setlength{\tabcolsep}{4pt}
    \setlength{\tabcolsep}{4pt} % Shrink horizontal space
    \renewcommand{\arraystretch}{0.9} % Shrink row height
    \caption{Best Selected Parameter Levels for Problem with 100 Variables}
    \label{tab:best_parameters_100vars}
    \begin{tabular}{p{2cm} p{11cm}} % Two columns: Algorithm Name & Parameter Settings
        \toprule
        \textbf{Algorithm} & \textbf{Selected Parameter Values Based on the TOPSIS Method} \\
        \midrule
        \multirow{8}{*}{BRADO}  
        & Threshold parameter ($\alpha$): 12 \\
        & Best neighbor weight (WG): 0.8 \\
        & Distance from the worst destination node (D): 0.25 \\
        & Initial population ($P_0$): 100 \\
        & Probability P in ER model: 0.8 \\
        & Probability of returning to origin country: 0.1 \\
        & Number of initial countries: 7 \\
        & Maximum iterations without improvement: 150 \\
        \midrule
        \multirow{4}{*}{GA}  
        & Maximum iterations without improvement: 30 \\
        & Initial population: 30 \\
        & Crossover probability: 0.1 \\
        & Survival rate of the population: 0.5 \\
        \midrule
        \multirow{7}{*}{ICA}  
        & Revolution rate values: 0.5 \\
        & Uniting threshold values: 0.01 \\
        & Zeta values: 0.04 \\
        & Population size values: 90 \\
        & Assimilation coefficient values: 1 \\
        & Number of initial imperialist values: 7 \\
        & Maximum iterations without improvement: 100 \\
        \midrule
        \multirow{4}{*}{ILS}  
        & Initial node selection method: 1 \\
        & Maximum iterations without improvement: 150 \\
        & Perturbation radius for new point: 1 \\
        & Number of iterations: 20 \\
        \midrule
        \multirow{2}{*}{LS}  
        & Maximum iterations without improvement: 30 \\
        & Perturbation radius for new point: 0.2 \\
        \midrule
        \multirow{3}{*}{MLS}  
        & Maximum iterations without improvement: 100 \\
        & Perturbation radius for new point: 1 \\
        & Number of iterations: 20 \\
        \midrule
        \multirow{4}{*}{PSO}  
        & Maximum iterations without improvement: 100 \\
        & Initial population: 100 \\
        & $C$ (cognitive parameter): 1 \\
        & $C$ (social parameter): 0.5 \\
        \bottomrule
    \end{tabular}
\end{table}

\begin{table}[!htb]
    \centering
    \small
    \setlength{\tabcolsep}{4pt}
    \setlength{\tabcolsep}{4pt} % Shrink horizontal space
    \renewcommand{\arraystretch}{0.9} % Shrink row height
    \caption{Best Selected Parameter Levels for Problem with 200 Variables}
    \label{tab:best_parameters_200vars}
    \begin{tabular}{p{2cm} p{11cm}} % Two columns: Algorithm Name & Parameter Settings
        \toprule
        \textbf{Algorithm} & \textbf{Selected Parameter Values Based on the TOPSIS Method} \\
        \midrule
        \multirow{8}{*}{BRADO}  
        & Threshold parameter ($\alpha$): 20 \\
        & Best neighbor weight (WG): 0.8 \\
        & Distance from the worst destination node (D): 0.2 \\
        & Initial population ($P_0$): 70 \\
        & Probability P in ER model: 0.8 \\
        & Probability of returning to origin country: 0.2 \\
        & Number of initial countries: 8 \\
        & Maximum iterations without improvement: 150 \\
        \midrule
        \multirow{4}{*}{GA}  
        & Maximum iterations without improvement: 150 \\
        & Initial population: 30 \\
        & Crossover probability: 0.1 \\
        & Survival rate of the population: 0.4 \\
        \midrule
        \multirow{7}{*}{ICA}  
        & Revolution rate values: 0.3 \\
        & Uniting threshold values: 0.01 \\
        & Zeta values: 0.01 \\
        & Population size values: 100 \\
        & Assimilation coefficient values: 1 \\
        & Number of initial imperialist values: 7 \\
        & Maximum iterations without improvement: 150 \\
        \midrule
        \multirow{4}{*}{ILS}  
        & Initial node selection method: 1 \\
        & Maximum iterations without improvement: 150 \\
        & Perturbation radius for new point: 1 \\
        & Number of iterations: 20 \\
        \midrule
        \multirow{2}{*}{LS}  
        & Maximum iterations without improvement: 30 \\
        & Perturbation radius for new point: 0.2 \\
        \midrule
        \multirow{3}{*}{MLS}  
        & Maximum iterations without improvement: 150 \\
        & Perturbation radius for new point: 1 \\
        & Number of iterations: 5 \\
        \midrule
        \multirow{4}{*}{PSO}  
        & Maximum iterations without improvement: 150 \\
        & Initial population: 50 \\
        & $C$ (cognitive parameter): 1.5 \\
        & $C$ (social parameter): 1.5 \\
        \bottomrule
    \end{tabular}
\end{table}

\begin{table}[!htb]
    \centering
    \caption{Best Selected Parameter Levels for Problem with 300 Variables}
    \label{tab:best_parameters_300vars}
    \small
    \setlength{\tabcolsep}{4pt}
    \setlength{\tabcolsep}{4pt} % Shrink horizontal space
    \renewcommand{\arraystretch}{0.9} % Shrink row height
    \begin{tabular}{p{2cm} p{11cm}} % Two columns: Algorithm Name & Parameter Settings
        \toprule
        \textbf{Algorithm} & \textbf{Selected Parameter Values Based on the TOPSIS Method} \\
        \midrule
        \multirow{8}{*}{BRADO}  
        & Threshold parameter ($\alpha$): 12 \\
        & Best neighbor weight (WG): 0.8 \\
        & Distance from the worst destination node (D): 0.2 \\
        & Initial population ($P_0$): 100 \\
        & Probability P in ER model: 0.8 \\
        & Probability of returning to origin country: 0.1 \\
        & Number of initial countries: 6 \\
        & Maximum iterations without improvement: 150 \\
        \midrule
        \multirow{4}{*}{GA}  
        & Maximum iterations without improvement: 150 \\
        & Initial population: 30 \\
        & Crossover probability: 0.1 \\
        & Survival rate of the population: 0.4 \\
        \midrule
        \multirow{7}{*}{ICA}  
        & Revolution rate values: 0.2 \\
        & Uniting threshold values: 0.01 \\
        & Zeta values: 0.04 \\
        & Population size values: 100 \\
        & Assimilation coefficient values: 2 \\
        & Number of initial imperialist values: 5 \\
        & Maximum iterations without improvement: 150 \\
        \midrule
        \multirow{4}{*}{ILS}  
        & Initial node selection method: 1 \\
        & Maximum iterations without improvement: 70 \\
        & Perturbation radius for new point: 1 \\
        & Number of iterations: 15 \\
        \midrule
        \multirow{2}{*}{LS}  
        & Maximum iterations without improvement: 30 \\
        & Perturbation radius for new point: 0.2 \\
        \midrule
        \multirow{3}{*}{MLS}  
        & Maximum iterations without improvement: 30 \\
        & Perturbation radius for new point: 1 \\
        & Number of iterations: 5 \\
        \midrule
        \multirow{4}{*}{PSO}  
        & Maximum iterations without improvement: 70 \\
        & Initial population: 80 \\
        & $C$ (cognitive parameter): 2 \\
        & $C$ (social parameter): 1.5 \\
        \bottomrule
    \end{tabular}
\end{table}

\begin{table}[!htb]
    \centering
    \small
    \setlength{\tabcolsep}{4pt}
    \setlength{\tabcolsep}{4pt} % Shrink horizontal space
    \renewcommand{\arraystretch}{0.9} % Shrink row height
    \caption{Best Selected Parameter Levels for Problem with 500 Variables}
    \label{tab:best_parameters_500vars}
    \begin{tabular}{p{2cm} p{11cm}} % Two columns: Algorithm Name & Parameter Settings
        \toprule
        \textbf{Algorithm} & \textbf{Selected Parameter Values Based on the TOPSIS Method} \\
        \midrule
        \multirow{8}{*}{BRADO}  
        & Threshold parameter ($\alpha$): 10 \\
        & Best neighbor weight (WG): 0.8 \\
        & Distance from the worst destination node (D): 0.25 \\
        & Initial population ($P_0$): 100 \\
        & Probability P in ER model: 0.8 \\
        & Probability of returning to origin country: 0.1 \\
        & Number of initial countries: 5 \\
        & Maximum iterations without improvement: 150 \\
        \midrule
        \multirow{4}{*}{GA}  
        & Maximum iterations without improvement: 150 \\
        & Initial population: 30 \\
        & Crossover probability: 0.1 \\
        & Survival rate of the population: 0.5 \\
        \midrule
        \multirow{7}{*}{ICA}  
        & Revolution rate values: 0.4 \\
        & Uniting threshold values: 0.03 \\
        & Zeta values: 0.04 \\
        & Population size values: 90 \\
        & Assimilation coefficient values: 2 \\
        & Number of initial imperialist values: 6 \\
        & Maximum iterations without improvement: 150 \\
        \midrule
        \multirow{4}{*}{ILS}  
        & Initial node selection method: 2 \\
        & Maximum iterations without improvement: 70 \\
        & Perturbation radius for new point: 1 \\
        & Number of iterations: 5 \\
        \midrule
        \multirow{2}{*}{LS}  
        & Maximum iterations without improvement: 30 \\
        & Perturbation radius for new point: 0.2 \\
        \midrule
        \multirow{3}{*}{MLS}  
        & Maximum iterations without improvement: 30 \\
        & Perturbation radius for new point: 1 \\
        & Number of iterations: 5 \\
        \midrule
        \multirow{4}{*}{PSO}  
        & Maximum iterations without improvement: 70 \\
        & Initial population: 80 \\
        & $C$ (cognitive parameter): 2 \\
        & $C$ (social parameter): 1 \\
        \bottomrule
    \end{tabular}
\end{table}

\begin{table}[!htb]
    \centering
    \caption{Best Selected Parameter Levels for Problem with 1000 Variables}
    \label{tab:best_parameters_1000vars}
    \small
    \setlength{\tabcolsep}{4pt}
    \setlength{\tabcolsep}{4pt} % Shrink horizontal space
    \renewcommand{\arraystretch}{0.9} % Shrink row height
    \begin{tabular}{p{2cm} p{11cm}} % Two columns: Algorithm Name & Parameter Settings
        \toprule
        \textbf{Algorithm} & \textbf{Selected Parameter Values Based on the TOPSIS Method} \\
        \midrule
        \multirow{8}{*}{BRADO}  
        & Threshold parameter ($\alpha$): 10\\
        & Best neighbor weight (WG): 0.8 \\
        & Distance from the worst destination node (D): 0.15 \\
        & Initial population ($P_0$): 70 \\
        & Probability P in ER model: 0.9 \\
        & Probability of returning to origin country: 0.1 \\
        & Number of initial countries: 6 \\
        & Maximum iterations without improvement: 150 \\
        \midrule
        \multirow{4}{*}{GA}  
        & Maximum iterations without improvement: 70 \\
        & Initial population: 30 \\
        & Crossover probability: 0.1 \\
        & Survival rate of the population: 0.4 \\
        \midrule
        \multirow{7}{*}{ICA}  
        & Revolution rate values: 0.04 \\
        & Uniting threshold values: 0.04 \\
        & Zeta values: 0.03 \\
        & Population size values: 90 \\
        & Assimilation coefficient values: 2 \\
        & Number of initial imperialist values: 5 \\
        & Maximum iterations without improvement: 100 \\
        \midrule
        \multirow{4}{*}{ILS}  
        & Initial node selection method: 2 \\
        & Maximum iterations without improvement: 30 \\
        & Perturbation radius for new point: 1 \\
        & Number of iterations: 5 \\
        \midrule
        \multirow{2}{*}{LS}  
        & Maximum iterations without improvement: 30 \\
        & Perturbation radius for new point: 0.5 \\
        \midrule
        \multirow{3}{*}{MLS}  
        & Maximum iterations without improvement: 30 \\
        & Perturbation radius for new point: 1 \\
        & Number of iterations: 5 \\
        \midrule
        \multirow{4}{*}{PSO}  
        & Maximum iterations without improvement: 70 \\
        & Initial population: 30 \\
        & $C$ (cognitive parameter): 1 \\
        & $C$ (social parameter): 2 \\
        \bottomrule
    \end{tabular}
\end{table}

After determining the optimal values for each parameter, the algorithms were executed 10 times using the optimized parameters. The best, worst, and average values of the objective function cost and NFE (Number of Function Evaluations) were recorded, as shown below.

\begin{table}[!htb]
    \centering
    \renewcommand{\arraystretch}{1.2} % Adjust row height for better readability
    \caption{Execution Results for 8-Queens}
    \label{tab:execution_results_8vars}
    \begin{tabular}{l l c c c}
        \toprule
        \textbf{Algorithm} & \textbf{Metric} & \textbf{Min} & \textbf{AVG} & \textbf{MAX} \\
        \midrule
        \multirow{2}{*}{BRADO}  
        & Cost & 0 & 3 & 7 \\
        & NFE  & 16560 & 53271 & 69930 \\
        \midrule
        \multirow{2}{*}{GA}  
        & Cost & 0 & 0.4 & 1 \\
        & NFE  & 7900 & 8975 & 10050 \\
        \midrule
        \multirow{2}{*}{ICA}  
        & Cost & 0 & 0.8 & 1 \\
        & NFE  & 8346 & 9902 & 13467 \\
        \midrule
        \multirow{2}{*}{ILS}  
        & Cost & 1 & 1.8 & 3 \\
        & NFE  & 1708 & 2071.4 & 2279 \\
        \midrule
        \multirow{2}{*}{LS}  
        & Cost & 1 & 4.8 & 7 \\
        & NFE  & 159 & 183 & 283 \\
        \midrule
        \multirow{2}{*}{MLS}  
        & Cost & 0 & 1.6 & 3 \\
        & NFE  & 3742 & 4166.1 & 4537 \\
        \midrule
        \multirow{2}{*}{PSO}  
        & Cost & 0 & 1.1 & 2 \\
        & NFE  & 3200 & 4310 & 6500 \\
        \bottomrule
    \end{tabular}
\end{table}

\begin{table}[!htb]
    \centering
    \renewcommand{\arraystretch}{1.2} % Adjust row height for better readability
    \caption{Execution Results for 10-Queens}
    \label{tab:execution_results_10vars}
    \begin{tabular}{l l c c c}
        \toprule
        \textbf{Algorithm} & \textbf{Metric} & \textbf{Min} & \textbf{AVG} & \textbf{MAX} \\
        \midrule
        \multirow{2}{*}{BRADO}  
        & Cost & 1 & 2.6 & 7 \\
        & NFE  & 16470 & 75159 & 103950 \\
        \midrule
        \multirow{2}{*}{GA}  
        & Cost & 0 & 0.4 & 1 \\
        & NFE  & 15700 & 19130 & 29000 \\
        \midrule
        \multirow{2}{*}{ICA}  
        & Cost & 1 & 1.1 & 2 \\
        & NFE  & 11468 & 15119 & 23506 \\
        \midrule
        \multirow{2}{*}{ILS}  
        & Cost & 1 & 3.3 & 6 \\
        & NFE  & 1505 & 1630.3 & 1883 \\
        \midrule
        \multirow{2}{*}{LS}  
        & Cost & 5 & 6.5 & 9 \\
        & NFE  & 153 & 196.4 & 246 \\
        \midrule
        \multirow{2}{*}{MLS}  
        & Cost & 1 & 2.3 & 3 \\
        & NFE  & 2878 & 3283.4 & 3638 \\
        \midrule
        \multirow{2}{*}{PSO}  
        & Cost & 0 & 2.5 & 4 \\
        & NFE  & 10500 & 12270 & 15600 \\
        \bottomrule
    \end{tabular}
\end{table}

\begin{table}[!htb]
    \centering
    \renewcommand{\arraystretch}{1.2} % Adjust row height for better readability
    \caption{Execution Results for 25-Queens}
    \label{tab:execution_results_25vars}
    \begin{tabular}{l l c c c}
        \toprule
        \textbf{Algorithm} & \textbf{Metric} & \textbf{Min} & \textbf{AVG} & \textbf{MAX} \\
        \midrule
        \multirow{2}{*}{BRADO}  
        & Cost & 1 & 1.9 & 4 \\
        & NFE  & 42160 & 63304 & 81920 \\
        \midrule
        \multirow{2}{*}{GA}  
        & Cost & 2 & 3.2 & 5 \\
        & NFE  & 9060 & 11757 & 19800 \\
        \midrule
        \multirow{2}{*}{ICA}  
        & Cost & 7 & 8.6 & 11 \\
        & NFE  & 9856 & 15719 & 24206 \\
        \midrule
        \multirow{2}{*}{ILS}  
        & Cost & 10 & 15.5 & 19 \\
        & NFE  & 3368 & 3943 & 4800 \\
        \midrule
        \multirow{2}{*}{LS}  
        & Cost & 15 & 22.2 & 35 \\
        & NFE  & 190 & 325.2 & 453 \\
        \midrule
        \multirow{2}{*}{MLS}  
        & Cost & 11 & 13.9 & 17 \\
        & NFE  & 4315 & 4683.7 & 5249 \\
        \midrule
        \multirow{2}{*}{PSO}  
        & Cost & 7 & 10.5 & 15 \\
        & NFE  & 9300 & 12720 & 18400 \\
        \bottomrule
    \end{tabular}
\end{table}

\begin{table}[!htb]
    \centering
    \renewcommand{\arraystretch}{1.2} % Adjust row height for better readability
    \caption{Execution Results for for 50-Queens}
    \label{tab:execution_results_50vars}
    \begin{tabular}{l l c c c}
        \toprule
        \textbf{Algorithm} & \textbf{Metric} & \textbf{Min} & \textbf{AVG} & \textbf{MAX} \\
        \midrule
        \multirow{2}{*}{BRADO}  
        & Cost & 1 & 1.8 & 3 \\
        & NFE  & 46130 & 60557 & 74830 \\
        \midrule
        \multirow{2}{*}{GA}  
        & Cost & 17 & 20.9 & 29 \\
        & NFE  & 5760 & 12222 & 16800 \\
        \midrule
        \multirow{2}{*}{ICA}  
        & Cost & 20 & 26.5 & 32 \\
        & NFE  & 16058 & 24554 & 40055 \\
        \midrule
        \multirow{2}{*}{ILS}  
        & Cost & 34 & 37.5 & 46 \\
        & NFE  & 4290 & 5182.2 & 6130 \\
        \midrule
        \multirow{2}{*}{LS}  
        & Cost & 40 & 57.3 & 76 \\
        & NFE  & 90 & 182.5 & 285 \\
        \midrule
        \multirow{2}{*}{MLS}  
        & Cost & 27 & 38.4 & 46 \\
        & NFE  & 6026 & 7006 & 7805 \\
        \midrule
        \multirow{2}{*}{PSO}  
        & Cost & 24 & 27 & 35 \\
        & NFE  & 13500 & 17650 & 24000 \\
        \bottomrule
    \end{tabular}
\end{table}

\begin{table}[!htb]
    \centering
    \renewcommand{\arraystretch}{1.2} % Adjust row height for better readability
    \caption{Execution Results for 100-Queens}
    \label{tab:execution_results_100vars}
    \begin{tabular}{l l c c c}
        \toprule
        \textbf{Algorithm} & \textbf{Metric} & \textbf{Min} & \textbf{AVG} & \textbf{MAX} \\
        \midrule
        \multirow{2}{*}{BRADO}  
        & Cost & 0 & 2.9 & 15 \\
        & NFE  & 72200 & 93210 & 115000 \\
        \midrule
        \multirow{2}{*}{GA}  
        & Cost & 77 & 86.3 & 96 \\
        & NFE  & 1620 & 2742 & 3990 \\
        \midrule
        \multirow{2}{*}{ICA}  
        & Cost & 61 & 65.7 & 70 \\
        & NFE  & 24714 & 31457 & 35854 \\
        \midrule
        \multirow{2}{*}{ILS}  
        & Cost & 87 & 95 & 103 \\
        & NFE  & 6601 & 8071.4 & 9310 \\
        \midrule
        \multirow{2}{*}{LS}  
        & Cost & 116 & 150.8 & 180 \\
        & NFE  & 31 & 52.1 & 104 \\
        \midrule
        \multirow{2}{*}{MLS}  
        & Cost & 95 & 100.6 & 114 \\
        & NFE  & 4434 & 5500.4 & 6544 \\
        \midrule
        \multirow{2}{*}{PSO}  
        & Cost & 75 & 84.2 & 91 \\
        & NFE  & 18100 & 27300 & 38800 \\
        \bottomrule
    \end{tabular}
\end{table}

\begin{table}[!htb]
    \centering
    \renewcommand{\arraystretch}{1.2} % Adjust row height for better readability
    \caption{Execution Results for 200-Queens}
    \label{tab:execution_results_200vars}
    \begin{tabular}{l l c c c}
        \toprule
        \textbf{Algorithm} & \textbf{Metric} & \textbf{Min} & \textbf{AVG} & \textbf{MAX} \\
        \midrule
        \multirow{2}{*}{BRADO}  
        & Cost & 1 & 4.3 & 25 \\
        & NFE  & 53550 & 76489 & 186620 \\
        \midrule
        \multirow{2}{*}{GA}  
        & Cost & 184 & 194.5 & 208 \\
        & NFE  & 7290 & 10635 & 16110 \\
        \midrule
        \multirow{2}{*}{ICA}  
        & Cost & 161 & 171.6 & 182 \\
        & NFE  & 35715 & 41736 & 50574 \\
        \midrule
        \multirow{2}{*}{ILS}  
        & Cost & 215 & 230.1 & 256 \\
        & NFE  & 6733 & 8207.7 & 9632 \\
        \midrule
        \multirow{2}{*}{LS}  
        & Cost & 285 & 315.3 & 375 \\
        & NFE  & 35 & 68.1 & 169 \\
        \midrule
        \multirow{2}{*}{MLS}  
        & Cost & 213 & 237.3 & 266 \\
        & NFE  & 1861 & 2366 & 3032 \\
        \midrule
        \multirow{2}{*}{PSO}  
        & Cost & 188 & 191 & 193 \\
        & NFE  & 12400 & 22285 & 40350 \\
        \bottomrule
    \end{tabular}
\end{table}

\begin{table}[!htb]
    \centering
    \renewcommand{\arraystretch}{1.2} % Adjust row height for better readability
    \caption{Execution Results for Problem with 300 Variables}
    \label{tab:execution_results_300vars}
    \begin{tabular}{l l c c c}
        \toprule
        \textbf{Algorithm} & \textbf{Metric} & \textbf{Min} & \textbf{AVG} & \textbf{MAX} \\
        \midrule
        \multirow{2}{*}{BRADO}  
        & Cost & 1 & 6.6 & 48 \\
        & NFE  & 60900 & 111890 & 386100 \\
        \midrule
        \multirow{2}{*}{GA}  
        & Cost & 288 & 312.3 & 325 \\
        & NFE  & 6150 & 15210 & 25860 \\
        \midrule
        \multirow{2}{*}{ICA}  
        & Cost & 271 & 281.3 & 286 \\
        & NFE  & 27830 & 40580 & 63492 \\
        \midrule
        \multirow{2}{*}{ILS}  
        & Cost & 356 & 379.8 & 412 \\
        & NFE  & 2641 & 3074.4 & 3629 \\
        \midrule
        \multirow{2}{*}{LS}  
        & Cost & 439 & 490.3 & 527 \\
        & NFE  & 37 & 64 & 119 \\
        \midrule
        \multirow{2}{*}{MLS}  
        & Cost & 382 & 425.6 & 461 \\
        & NFE  & 289 & 452.3 & 647 \\
        \midrule
        \multirow{2}{*}{PSO}  
        & Cost & 285 & 286.8 & 289 \\
        & NFE  & 13040 & 21792 & 26960 \\
        \bottomrule
    \end{tabular}
\end{table}

\begin{table}[!htb]
    \centering
    \renewcommand{\arraystretch}{1.2} % Adjust row height for better readability
    \caption{Execution Results for 500-Queens}
    \label{tab:execution_results_500vars}
    \begin{tabular}{l l c c c}
        \toprule
        \textbf{Algorithm} & \textbf{Metric} & \textbf{Min} & \textbf{AVG} & \textbf{MAX} \\
        \midrule
        \multirow{2}{*}{BRADO}  
        & Cost & 1 & 9.1 & 72 \\
        & NFE  & 57300 & 154270 & 752200 \\
        \midrule
        \multirow{2}{*}{GA}  
        & Cost & 544 & 581.8 & 619 \\
        & NFE  & 6990 & 22473 & 43680 \\
        \midrule
        \multirow{2}{*}{ICA}  
        & Cost & 476 & 483.5 & 488 \\
        & NFE  & 26529 & 35785 & 48321 \\
        \midrule
        \multirow{2}{*}{ILS}  
        & Cost & 710 & 764 & 811 \\
        & NFE  & 435 & 698.8 & 1228 \\
        \midrule
        \multirow{2}{*}{LS}  
        & Cost & 759 & 819.1 & 878 \\
        & NFE  & 40 & 80 & 134 \\
        \midrule
        \multirow{2}{*}{MLS}  
        & Cost & 691 & 730.7 & 783 \\
        & NFE  & 214 & 421.9 & 675 \\
        \midrule
        \multirow{2}{*}{PSO}  
        & Cost & 481 & 487.4 & 491 \\
        & NFE  & 7840 & 8608 & 9120 \\
        \bottomrule
    \end{tabular}
\end{table}

\begin{table}[!htb]
    \centering
    \renewcommand{\arraystretch}{1.2} % Adjust row height for better readability
    \caption{Execution Results for 1000-Queens}
    \label{tab:execution_results_1000vars}
    \begin{tabular}{l l c c c}
        \toprule
        \textbf{Algorithm} & \textbf{Metric} & \textbf{Min} & \textbf{AVG} & \textbf{MAX} \\
        \midrule
        \multirow{2}{*}{BRADO}  
        & Cost & 1 & 21.8 & 198 \\
        & NFE  & 43330 & 124383 & 700700 \\
        \midrule
        \multirow{2}{*}{GA}  
        & Cost & 1292 & 1332.5 & 1355 \\
        & NFE  & 4260 & 6540 & 10530 \\
        \midrule
        \multirow{2}{*}{ICA}  
        & Cost & 974 & 980.1 & 989 \\
        & NFE  & 182275 & 35736 & 45403 \\
        \midrule
        \multirow{2}{*}{ILS}  
        & Cost & 1477 & 1574.1 & 1636 \\
        & NFE  & 216 & 266.7 & 391 \\
        \midrule
        \multirow{2}{*}{LS}  
        & Cost & 1572 & 1630.6 & 1742 \\
        & NFE  & 39 & 86.3 & 143 \\
        \midrule
        \multirow{2}{*}{MLS}  
        & Cost & 1525 & 1574 & 1611 \\
        & NFE  & 383 & 438.5 & 538 \\
        \midrule
        \multirow{2}{*}{PSO}  
        & Cost & 978 & 986.5 & 993 \\
        & NFE  & 2730 & 3096 & 3750 \\
        \bottomrule
    \end{tabular}
\end{table}

\end{document}
